# Supplementary material for: CPGAN: Full-Spectrum Content-Parsing Generative Adversarial Networks for Text-to-Image Synthesis
Source: arXiv:1912.08562 source file (2020-07-12)
Supplement: Supplementary file 1 [file 5_supplement_material.tex]

\section{Details of Coarse-to-fine Generative Framework}

As described in Sec 3.1 in the paper, we adopt three cascaded generators to obtain coarse-to-fine synthesized images. At each stage, the generator $G_i$ is adopted to generate intermediate feature maps $\mathbf{C_i}$ which could be directly mapped to generated image by convolutional layers.

\begin{figure}[t]
\centering
\includegraphics[height=3.5cm]{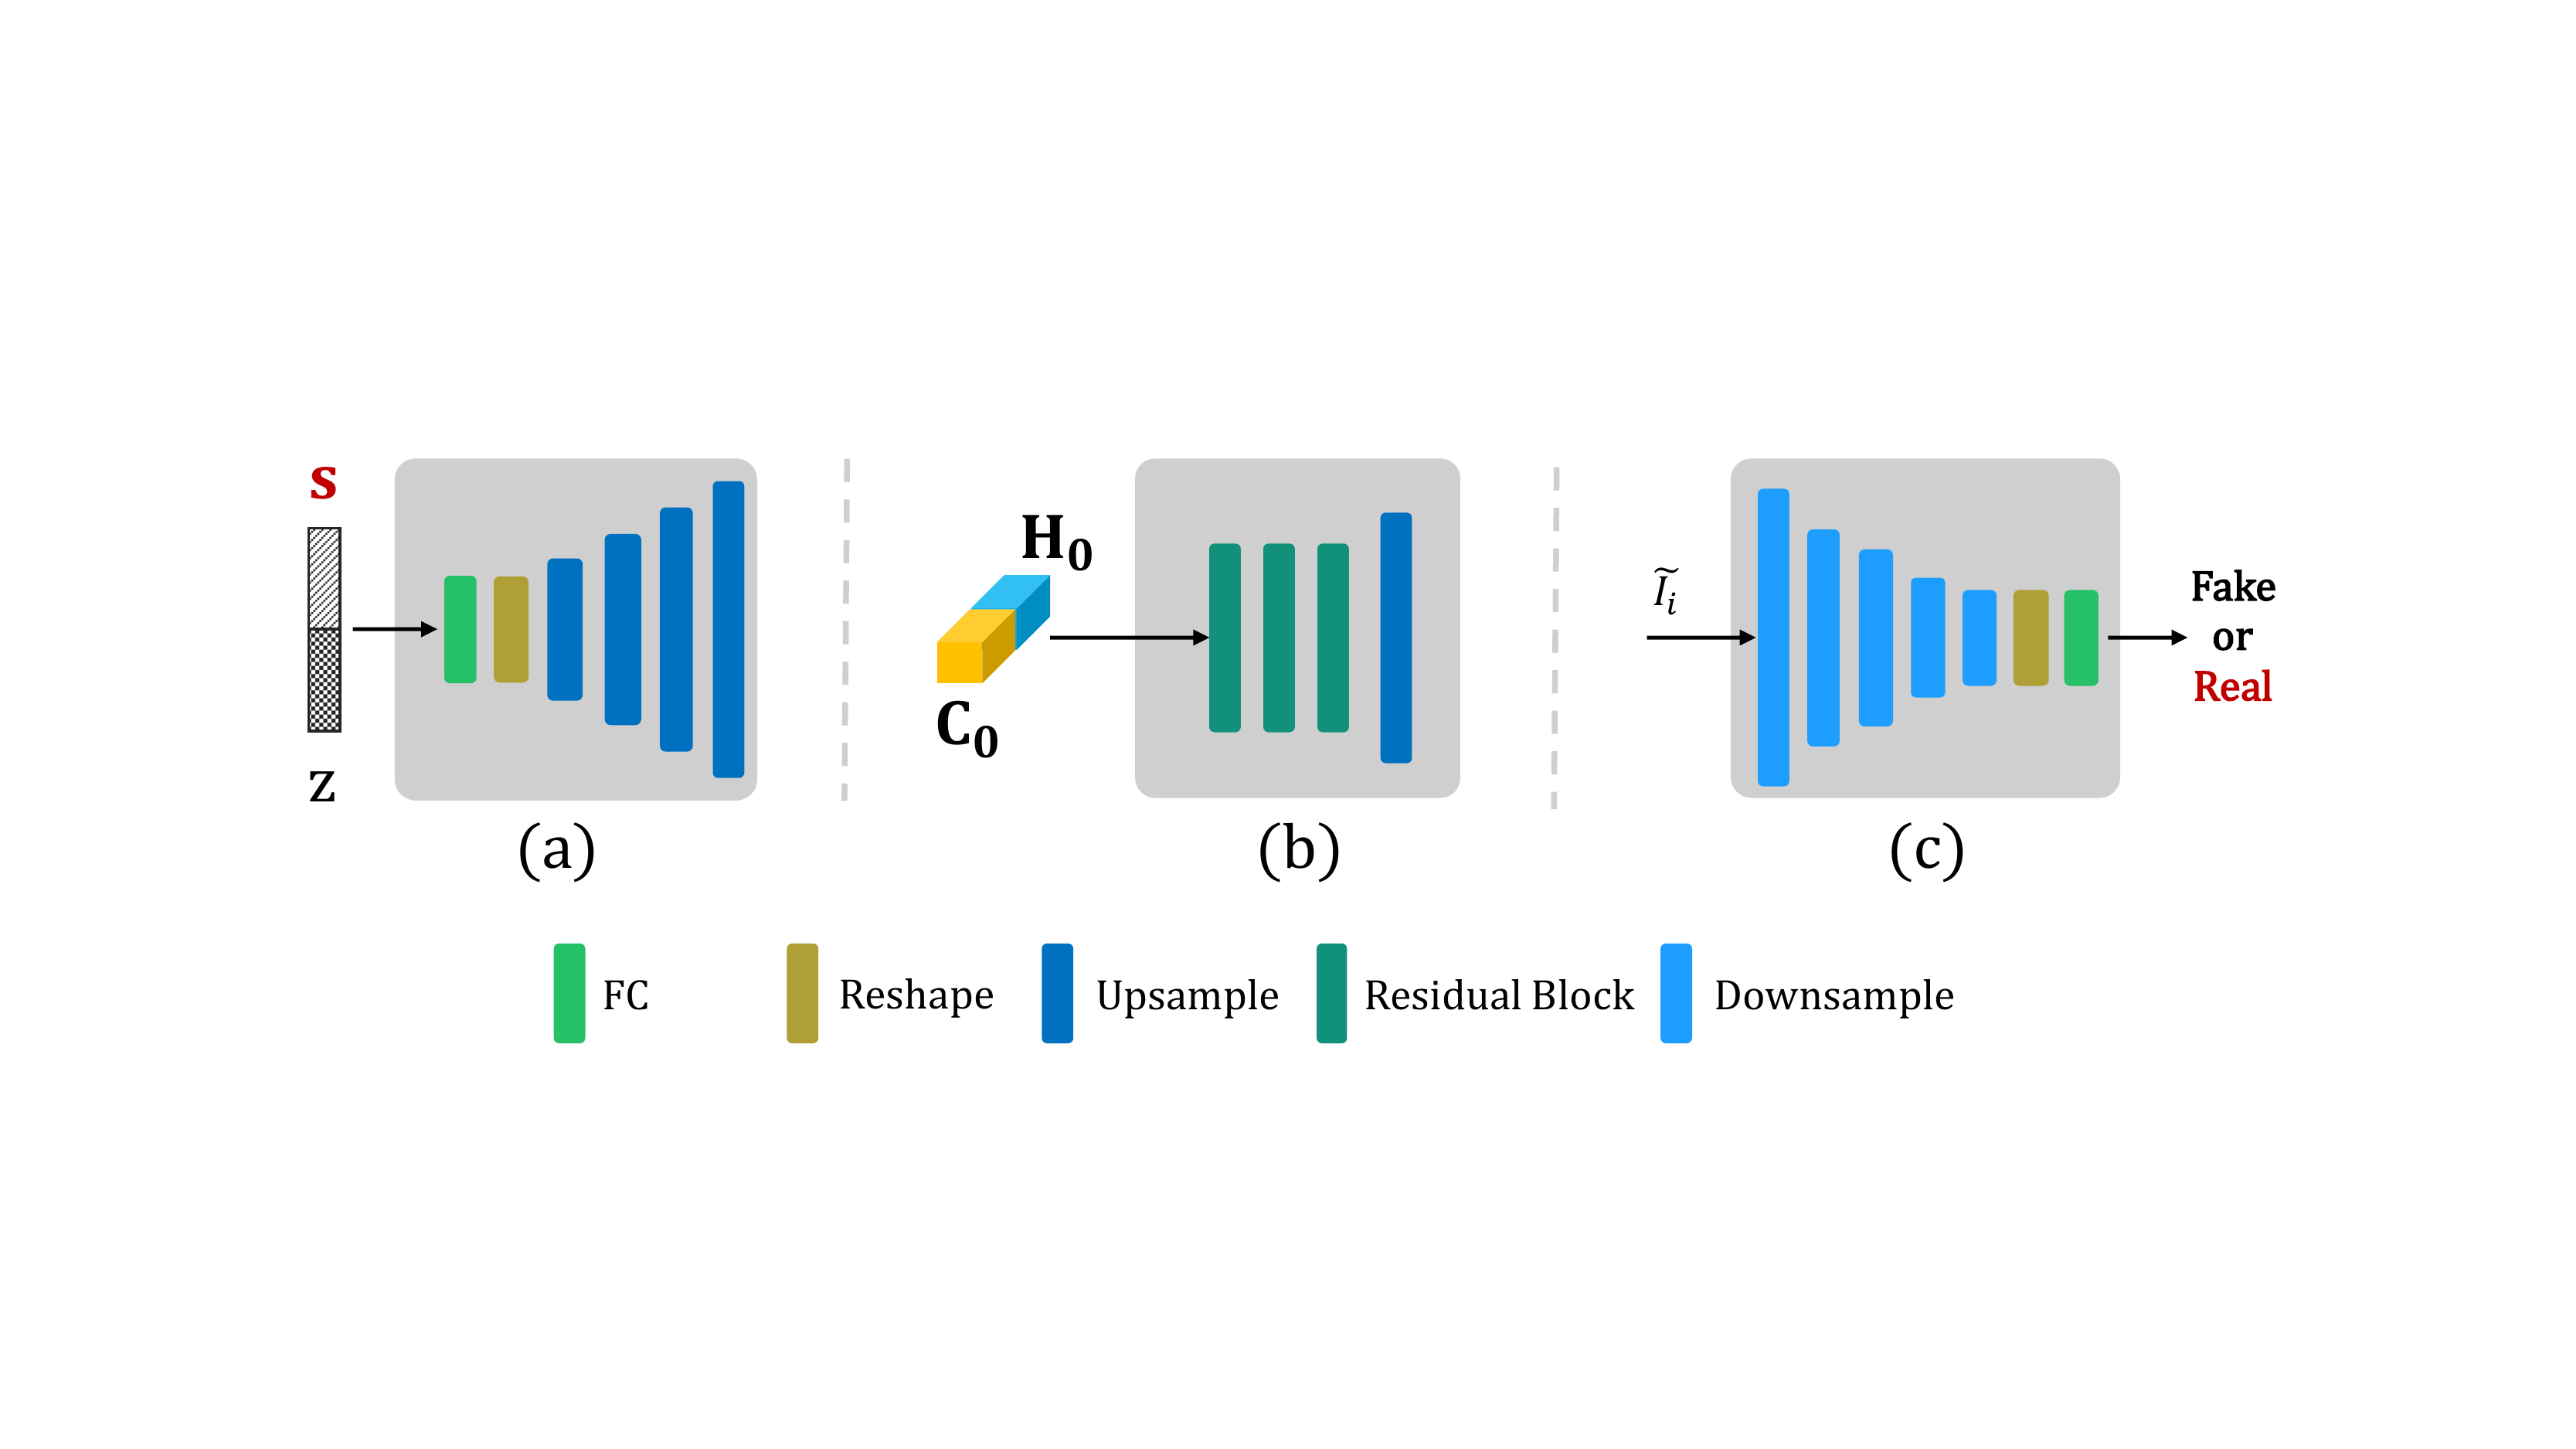}
\caption{Illustration of the coarse-to-fine framework of our CPGAN: (a) the structure of the initial generator $G_0$; (b) the structure of generators $G_1, G_2$; (c) the structure of unconditional discriminator.}
\label{fig:supplement}
\end{figure}

As shown in Figure~\ref{fig:supplement} (a), the global embedding for the whole sentence $\mathbf{s}$ concatenated with Gaussian noise $\mathbf{z}$ is processed by $G_0$, which is composed of a FC layer, a reshape layer and four cascaded upsampling layers. The obtain intermediate feature map $\mathbf{C_0}$, together with $\mathbf{H_0}$, are then fed into 
the subsequent generators $G_1$ and $G_2$, which consists of three residual blocks and a upsampling layer. 
Here $\mathbf{H_0}$ is the output of the attention model $F^{att}$ designed  to attend to the word embeddings $\mathbf{W}$ to each pixel of $\mathbf{C_0}$.
Formally, given the input word embedding $\mathbf{W} = \{\mathbf{w}_1, \mathbf{w}_2, \dots \mathbf{w}_T \}$ and the intermediate feature map $\mathbf{C_i} \in \mathbb{R}^{\hat{d} \times N_{i} \times N_{i}}$, the $\mathbf{H_i}$ is modeled as:
\begin{align}
    \mathbf{H_i} = F^{att}_i(\mathbf{W}, \mathbf{C_{i}}), \quad i=0, 1.
    \label{eqn:Fatt}
\end{align}
Herein $N_{i} \times N_{i}$ is the shape of intermediate feature map at the stage $i$ and $\mathbf{w}_t \in \mathbb{R}^{d}$ denotes the embedding for the $t$-th word.
The word embeddings are first projected into the common space of the intermediate features by a FC layer, $i.e., {\mathbf{\hat{w}}_t} = \mathbf{M}_{p}\mathbf{w}_{t}$, where $\mathbf{M}_{p} \in \mathbb{R}^{\hat{d} \times d}$.
Suppose the $(m,n)$-th intermediate feature in the feature map is denoted as $\mathbf{C_i}^{m,n} \in \mathbb{R}^{\hat{d}},m,n \in 1,2,3,...,N_{i}$.
We compute the dynamic representation of word embeddings related to the $(m,n)$-th intermediate feature by attention mechanism:
\begin{align}
\begin{split}
&b_k = \frac{\exp({(\mathbf{C_i}^{m,n})^{T} \mathbf{\hat{w}}_k})}{\sum_{p=1}^T \exp({(\mathbf{C_i}^{m,n})^{T} \mathbf{\hat{w}}_p})}, n=1, 2, \dots, T, \\
&\mathbf{H_i}^{m,n} = \sum_{k=1}^{T} b_k \mathbf{\hat{w}}_k,
\end{split}
\end{align}
where $\mathbf{H_i} \in \mathbb{R}^{\hat{d} \times N_i \times N_i}$ is the dynamic representation of word embeddings related to the intermediate feature maps $\mathbf{C_i}$.

\section{The Structure of Unconditional Discriminators}
The unconditional discriminator $D_i^{uc}$ in Sec 3.1 in the paper consists of five cascaded downsampling layers, a Reshape layer and a FC layer, as illustrated in Figure~\ref{fig:supplement} (c).

\section{DAMSM Loss}
We employ DAMSM~\cite{xu2018attngan} to construct our TISCL loss function for modeling the non-matching loss between a textual description $X$ and the corresponding synthesized image $\widetilde{I}$.
%As shown in Equation 13 in the main paper, the key difference between our TISCL and DAMSM lies in encoding mechanisms for both input text and the synthesized image .
Formally, given the final word embeddings $\mathbf{W} = \{\mathbf{w}_1, \mathbf{w}_2, \dots \mathbf{w}_T \}$ and sentence embedding $\mathbf{s}$ obtained by our text encoder in Equation 8 in the paper and the image embedding $\mathbf{V} \in \mathbb{R}^{256 \times 100}$ by our image encoder shown in Equation 9 in the paper, the TISCL is modeled as:
\begin{align}
\mathcal{L}_{\text{TISCL}} = \mathcal{L}_{\text{DAMSM}} (\mathbf{W}, \mathbf{s}, \mathbf{V}, \mathbf{f}).
\label{eqn:tiscl}
\end{align}
Here $\mathbf{f} \in \mathbb{R}^{d}$ is the image global feature extracted from the last average pooling layer of Inception-V3. 
We use $\mathbf{w}_T$ as the sentence embedding $\mathbf{s} \in \mathbb{R}^{d}$.

We first reshape $\mathbf{W}$ into matrix $\mathbf{\bar{W}} \in \mathbb{R}^{d \times T}$.
The similarity matrix for pairs of words and sub-regions is computed by:
\begin{align}
\mathbf{Sim} = (\mathbf{\bar{W}})^{T} \mathbf{V},
\end{align}
where $\mathbf{Sim}_{i,j}$ is the dot-product similarity between the $i$-th word of the sentence and the the $j$-th sub-region of the image.
We calculate the dynamic representation $\mathbf{c}_i$ for the word embedding $\mathbf{w}_i$ attending to the sub-regions of the image features by:

\begin{align}
\mathbf{\bar{Sim}}_{i,j} = \frac{\exp({\mathbf{Sim}_{i,j}) }}{\sum_{k=1}^{T} \exp({(\mathbf{Sim}_{k,j}})}, 
\end{align}

\begin{align}
\alpha_j = \frac{\exp({\gamma_1 \mathbf{\bar{Sim}}_{i,j}) }}{\sum_{k=1}^{100} \exp({(\gamma_1 \mathbf{\bar{Sim}}_{i,k}})}, 
\end{align}

\begin{align}
\mathbf{c}_i = \sum_{j=1}^{100} \alpha_j \mathbf{V}[:,j],
\end{align}
where $\gamma_1$ is a factor that determines how much attention is paid to features of its relevant sub-regions when computing
the region-context vector for a word.
Finally, we define the semantic consistency between each word of input text and different sub-region of the image using the cosine similarity, $i.e., R(\mathbf{c}_i,\mathbf{w}_i)=(\mathbf{c}_i^{T} \mathbf{w}_i)/(||\mathbf{c}_i||||\mathbf{w}_i||)$.
The image-text matching score between the entire image $\mathbf{I}$ and the whole sentence description $\textbf{D}$ is define as:
\begin{align}
R(\mathbf{I},\mathbf{D}) = \log(\sum_{i=1}^{T} \exp(\gamma_2 R(\mathbf{c}_i,\mathbf{w}_i)))^{1/\gamma_2},
\end{align}
where $\gamma_2$ is a factor that determines how much to magnify the importance of the most relevant word-to-region-context pair.

In a mini-batch of iteration, the posterior probability of sentence $\mathbf{D}_i$ matching with the corresponding image $\mathbf{I}_i$ is obtained by:
\begin{align}
P(\mathbf{D}_i|\mathbf{I}_i) = \frac{\exp(R(\gamma_3\mathbf{I}_i,\mathbf{D}_i))}{\sum_{j=1}^{M} \exp( R(\gamma_3\mathbf{I}_i,\mathbf{D}_j))},
\end{align}
where $\gamma_3$ is a smoothing factor determined by experiments. $M$ is batch size.
Then the word-level loss function of the positive image-sentence pair in a mini-batch is define as:
\begin{align}
	\mathcal{L}^{w} = -\sum_{i=1}^{M}\log P(\mathbf{D}_i|\mathbf{I}_i) + \log P(\mathbf{I}_i|\mathbf{D}_i)
\end{align}
For the sentence embedding $\mathbf{s}$ and the image global feature  $\mathbf{f}$, we define the image-text matching score by:
\begin{align}
\hat{R}(\mathbf{I},\mathbf{D}) = (\mathbf{f}^\top \mathbf{s})/ (||\mathbf{f}^\top||||\mathbf{s}||).
\end{align}
The sentence-level loss $\mathcal{L}^{s}$ is modeled as:
\begin{align}
\hat{P}(\mathbf{D}_i|\mathbf{I}_i) = \frac{\exp(\hat{R}(\gamma_3\mathbf{I}_i,\mathbf{D}_i))}{\sum_{j=1}^{M} \exp( \hat{R}(\gamma_3\mathbf{I}_i,\mathbf{D}_j))} 
\end{align}
\begin{align}
\mathcal{L}^{s} = -\sum_{i=1}^{M}\log \hat{P}(\mathbf{D}_i|\mathbf{I}_i) + \log \hat{P}(\mathbf{I}_i|\mathbf{D}_i)
\end{align}
Finally, the DAMSM loss is define as:
\begin{align}
\mathcal{L}_{DAMSM} = \mathcal{L}^{w} + \mathcal{L}^{s}
\end{align}
